# Supplementary material for: Constraining the $\Lambda\Lambda$ interaction with terrestrial and astronomical data
Source: arXiv:2602.18356 ancillary file (2026-02-20)
Supplement: Supplementary file 1 [file KIDS-LL-SM.pdf]

# Supplemental materials to "Constraining the $\Lambda\Lambda$ interaction in nuclei with terrestrial and astronomical data"

Yusuke Tanimura,[1] Chang Ho Hyun,[2] and Myung-Ki Cheoun[1]

[1] *Department of Physics and Origin of Matter and Evolution of Galaxies (OMEG) Institute, Soongsil University, Seoul 06978, Korea*

[2] *Department of Physics Education, Daegu University, Gyeongsan 38453, Korea*

(Dated: February 20, 2026)

**CONTENTS**

I. Parameter sets in $\Lambda\Lambda$ sector 1

II. Neutron-star properties 9

References 20

## I. PARAMETER SETS IN $\Lambda\Lambda$ SECTOR

See the main manuscript for details.

Tables I-VIII summarize KIDS-A-Y4-LL4($\lambda_2, \lambda_3$) parameter sets.

Tables IX-XIX summarize KIDS-D-Y4-LL4($\lambda_2, \lambda_3$) parameter sets.

TABLE I. KIDS-A-Y4-LL4($\lambda_2$,0) parameter sets. The MD value, which is independent of $\lambda_2$, is calculated for the full dataset of double-$\Lambda$ hypernuclei. We also indicate whether the maximum neutron-star mass exceeds $2M_\odot$ within the causal domain and whether the corresponding M-R relation is consistent with the NICER constraints ($2\sigma$ or $1\sigma$) for PSR J0740+6620 [1, 2].

| | KIDS-A-Y4-LL4($\lambda_2$,0) | | | | | | |
|---|---|---|---|---|---|---|---|
| $\lambda_0$ (MeVfm$^3$) | $-232.01$ | | | | | | |
| $\lambda_1$ (MeVfm$^5$) | 268.19 | | | | | | |
| $\lambda_2$ (MeVfm$^5$) | 0 | 100 | 200 | 300 | 400 | 500 | 600 |
| $\lambda_3$ (MeVfm$^6$) | 0 | | | | | | |
| MD (%) | 2.80 | | | | | | |
| $> 2M_\odot$ | no | no | no | yes | yes | yes | yes |
| J0740+6620 | no | no | $2\sigma$ | $2\sigma$ | $2\sigma$ | $1\sigma$ | $1\sigma$ |

TABLE II. Same as Table I, but for KIDS-A-Y4-LL4($\lambda_2$,100).

| | KIDS-A-Y4-LL4($\lambda_2$,100) | | | | | | |
|---|---|---|---|---|---|---|---|
| $\lambda_0$ (MeVfm$^3$) | $-259.26$ | | | | | | |
| $\lambda_1$ (MeVfm$^5$) | 298.60 | | | | | | |
| $\lambda_2$ (MeVfm$^5$) | 0 | 100 | 200 | 300 | 400 | 500 | 600 |
| $\lambda_3$ (MeVfm$^6$) | 100 | | | | | | |
| MD (%) | 2.88 | | | | | | |
| $> 2M_\odot$ | no | no | no | yes | yes | yes | yes |
| J0740+6620 | no | no | $2\sigma$ | $2\sigma$ | $2\sigma$ | $1\sigma$ | $1\sigma$ |

TABLE III. Same as Table I, but for KIDS-A-Y4-LL4($\lambda_2$,200).

| | KIDS-A-Y4-LL4($\lambda_2$,200) | | | | | | |
|---|---|---|---|---|---|---|---|
| $\lambda_0$ (MeVfm$^3$) | $-279.90$ | | | | | | |
| $\lambda_1$ (MeVfm$^5$) | 314.32 | | | | | | |
| $\lambda_2$ (MeVfm$^5$) | 0 | 100 | 200 | 300 | 400 | 500 | 600 |
| $\lambda_3$ (MeVfm$^6$) | 200 | | | | | | |
| MD (%) | 3.03 | | | | | | |
| $> 2M_\odot$ | no | no | no | yes | yes | yes | yes |
| J0740+6620 | no | no | $2\sigma$ | $2\sigma$ | $2\sigma$ | $1\sigma$ | $1\sigma$ |

TABLE IV. Same as Table I, but for KIDS-A-Y4-LL4($\lambda_2$,300).

| | KIDS-A-Y4-LL4($\lambda_2$,300) | | | | | | |
|---|---|---|---|---|---|---|---|
| $\lambda_0$ (MeVfm$^3$) | $-300.57$ | | | | | | |
| $\lambda_1$ (MeVfm$^5$) | 330.21 | | | | | | |
| $\lambda_2$ (MeVfm$^5$) | 0 | 100 | 200 | 300 | 400 | 500 | 600 |
| $\lambda_3$ (MeVfm$^6$) | 300 | | | | | | |
| MD (%) | 3.17 | | | | | | |
| $> 2M_\odot$ | no | no | no | yes | yes | yes | yes |
| J0740+6620 | no | no | $2\sigma$ | $2\sigma$ | $2\sigma$ | $1\sigma$ | $1\sigma$ |

TABLE V. Same as Table I, but for KIDS-A-Y4-LL4($\lambda_2$,400).

| | KIDS-A-Y4-LL4($\lambda_2$,400) | | | | | |
|---|---|---|---|---|---|---|
| $\lambda_0$ (MeVfm$^3$) | $-321.28$ | | | | | |
| $\lambda_1$ (MeVfm$^5$) | 346.31 | | | | | |
| $\lambda_2$ (MeVfm$^5$) | 0 | 100 | 200 | 300 | 400 | 500 |
| $\lambda_3$ (MeVfm$^6$) | 400 | | | | | |
| MD (%) | 3.32 | | | | | |
| $> 2M_\odot$ | no | no | no | yes | yes | yes |
| J0740+6620 | no | no | $2\sigma$ | $2\sigma$ | $1\sigma$ | $1\sigma$ |

TABLE VI. Same as Table I, but for KIDS-A-Y4-LL4($\lambda_2$,500).

| | KIDS-A-Y4-LL4($\lambda_2$,500) | | | | | |
|---|---|---|---|---|---|---|
| $\lambda_0$ (MeVfm$^3$) | $-342.05$ | | | | | |
| $\lambda_1$ (MeVfm$^5$) | 362.64 | | | | | |
| $\lambda_2$ (MeVfm$^5$) | 0 | 100 | 200 | 300 | 400 | 500 |
| $\lambda_3$ (MeVfm$^6$) | 500 | | | | | |
| MD (%) | 3.46 | | | | | |
| $> 2M_\odot$ | no | no | yes | yes | yes | yes |
| J0740+6620 | no | $2\sigma$ | $2\sigma$ | $2\sigma$ | $1\sigma$ | $1\sigma$ |

TABLE VII. Same as Table I, but for KIDS-A-Y4-LL4($\lambda_2$,600).

| | KIDS-A-Y4-LL4($\lambda_2$,600) | | | | |
|---|---|---|---|---|---|
| $\lambda_0$ (MeVfm$^3$) | $-362.96$ | | | | |
| $\lambda_1$ (MeVfm$^5$) | 379.47 | | | | |
| $\lambda_2$ (MeVfm$^5$) | 0 | 100 | 200 | 300 | 400 |
| $\lambda_3$ (MeVfm$^6$) | 600 | | | | |
| MD (%) | 3.60 | | | | |
| $> 2M_\odot$ | no | no | yes | yes | yes |
| J0740+6620 | no | $2\sigma$ | $2\sigma$ | $2\sigma$ | $1\sigma$ |

TABLE VIII. Same as Table I, but for KIDS-A-Y4-LL4($\lambda_2$,700).

| | KIDS-A-Y4-LL4($\lambda_2$,700) | | | | |
|---|---|---|---|---|---|
| $\lambda_0$ (MeVfm$^3$) | $-383.873$ | | | | |
| $\lambda_1$ (MeVfm$^5$) | 396.392 | | | | |
| $\lambda_2$ (MeVfm$^5$) | 0 | 100 | 200 | 300 | 400 |
| $\lambda_3$ (MeVfm$^6$) | 700 | | | | |
| MD (%) | 3.74 | | | | |
| $> 2M_\odot$ | no | no | yes | yes | yes |
| J0740+6620 | no | $2\sigma$ | $2\sigma$ | $2\sigma$ | $1\sigma$ |

TABLE IX. Same as Table I, but for KIDS-D-Y4-LL4($\lambda_2$,0).

| | KIDS-D-Y4-LL4($\lambda_2$,0) | | | | | | |
|---|---|---|---|---|---|---|---|
| $\lambda_0$ (MeVfm$^3$) | $-240.61$ | | | | | | |
| $\lambda_1$ (MeVfm$^5$) | 286.95 | | | | | | |
| $\lambda_2$ (MeVfm$^5$) | 0 | 100 | 200 | 300 | 400 | 500 | 600 |
| $\lambda_3$ (MeVfm$^6$) | 0 | | | | | | |
| MD (%) | 2.45 | | | | | | |
| $> 2M_\odot$ | no | no | yes | yes | yes | yes | yes |
| J0740+6620 | no | $2\sigma$ | $1\sigma$ | $1\sigma$ | $1\sigma$ | $1\sigma$ | $1\sigma$ |

TABLE X. Same as Table I, but for KIDS-D-Y4-LL4($\lambda_2$,100).

| | KIDS-D-Y4-LL4($\lambda_2$,100) | | | | | | |
|---|---|---|---|---|---|---|---|
| $\lambda_0$ (MeVfm$^3$) | $-261.55$ | | | | | | |
| $\lambda_1$ (MeVfm$^5$) | 302.90 | | | | | | |
| $\lambda_2$ (MeVfm$^5$) | 0 | 100 | 200 | 300 | 400 | 500 | 600 |
| $\lambda_3$ (MeVfm$^6$) | 100 | | | | | | |
| MD (%) | 2.34 | | | | | | |
| $> 2M_\odot$ | no | no | yes | yes | yes | yes | yes |
| J0740+6620 | no | $2\sigma$ | $1\sigma$ | $1\sigma$ | $1\sigma$ | $1\sigma$ | $1\sigma$ |

TABLE XI. Same as Table I, but for KIDS-D-Y4-LL4($\lambda_2$,200).

| | KIDS-D-Y4-LL4($\lambda_2$,200) | | | | | | |
|---|---|---|---|---|---|---|---|
| $\lambda_0$ (MeVfm$^3$) | $-287.87$ | | | | | | |
| $\lambda_1$ (MeVfm$^5$) | 331.36 | | | | | | |
| $\lambda_2$ (MeVfm$^5$) | 0 | 100 | 200 | 300 | 400 | 500 | 600 |
| $\lambda_3$ (MeVfm$^6$) | 200 | | | | | | |
| MD (%) | 2.41 | | | | | | |
| $> 2M_\odot$ | no | yes | yes | yes | yes | yes | yes |
| J0740+6620 | no | $2\sigma$ | $1\sigma$ | $1\sigma$ | $1\sigma$ | $1\sigma$ | $1\sigma$ |

TABLE XII. Same as Table I, but for KIDS-D-Y4-LL4($\lambda_2$,300).

| | KIDS-D-Y4-LL4($\lambda_2$,300) | | | | | | |
|---|---|---|---|---|---|---|---|
| $\lambda_0$ (MeVfm$^3$) | $-311.26$ | | | | | | |
| $\lambda_1$ (MeVfm$^5$) | 353.29 | | | | | | |
| $\lambda_2$ (MeVfm$^5$) | 0 | 100 | 200 | 300 | 400 | 500 | 600 |
| $\lambda_3$ (MeVfm$^6$) | 300 | | | | | | |
| MD (%) | 2.50 | | | | | | |
| $> 2M_\odot$ | no | yes | yes | yes | yes | yes | yes |
| J0740+6620 | no | $2\sigma$ | $1\sigma$ | $1\sigma$ | $1\sigma$ | $1\sigma$ | $1\sigma$ |

TABLE XIII. Same as Table I, but for KIDS-D-Y4-LL4($\lambda_2$,400).

| | KIDS-D-Y4-LL4($\lambda_2$,400) | | | | | | |
|---|---|---|---|---|---|---|---|
| $\lambda_0$ (MeVfm$^3$) | $-331.77$ | | | | | | |
| $\lambda_1$ (MeVfm$^5$) | 368.65 | | | | | | |
| $\lambda_2$ (MeVfm$^5$) | 0 | 100 | 200 | 300 | 400 | 500 | 600 |
| $\lambda_3$ (MeVfm$^6$) | 400 | | | | | | |
| MD (%) | 2.62 | | | | | | |
| $> 2M_\odot$ | no | yes | yes | yes | yes | yes | yes |
| J0740+6620 | no | $1\sigma$ | $1\sigma$ | $1\sigma$ | $1\sigma$ | $1\sigma$ | $1\sigma$ |

TABLE XIV. Same as Table I, but for KIDS-D-Y4-LL4($\lambda_2$,500).

| | KIDS-D-Y4-LL4($\lambda_2$,500) | | | | | | |
|---|---|---|---|---|---|---|---|
| $\lambda_0$ (MeVfm$^3$) | $-352.32$ | | | | | | |
| $\lambda_1$ (MeVfm$^5$) | 384.23 | | | | | | |
| $\lambda_2$ (MeVfm$^5$) | 0 | 100 | 200 | 300 | 400 | 500 | 600 |
| $\lambda_3$ (MeVfm$^6$) | 500 | | | | | | |
| MD (%) | 2.74 | | | | | | |
| $> 2M_\odot$ | no | yes | yes | yes | yes | yes | yes |
| J0740+6620 | no | $1\sigma$ | $1\sigma$ | $1\sigma$ | $1\sigma$ | $1\sigma$ | $1\sigma$ |

TABLE XV. Same as Table I, but for KIDS-D-Y4-LL4($\lambda_2$,600).

| | KIDS-D-Y4-LL4($\lambda_2$,600) | | | | | | |
|---|---|---|---|---|---|---|---|
| $\lambda_0$ (MeVfm$^3$) | −372.92 | | | | | | |
| $\lambda_1$ (MeVfm$^5$) | 400.01 | | | | | | |
| $\lambda_2$ (MeVfm$^5$) | 0 | 100 | 200 | 300 | 400 | 500 | 600 |
| $\lambda_3$ (MeVfm$^6$) | 600 | | | | | | |
| MD (%) | 2.86 | | | | | | |
| $> 2M_\odot$ | no | yes | yes | yes | yes | yes | yes |
| J0740+6620 | $2\sigma$ | $1\sigma$ | $1\sigma$ | $1\sigma$ | $1\sigma$ | $1\sigma$ | $1\sigma$ |

TABLE XVI. Same as Table I, but for KIDS-D-Y4-LL4($\lambda_2$,700).

| | KIDS-D-Y4-LL4($\lambda_2$,700) | | | | | | |
|---|---|---|---|---|---|---|---|
| $\lambda_0$ (MeVfm$^3$) | −393.57 | | | | | | |
| $\lambda_1$ (MeVfm$^5$) | 416.03 | | | | | | |
| $\lambda_2$ (MeVfm$^5$) | 0 | 100 | 200 | 300 | 400 | 500 | 600 |
| $\lambda_3$ (MeVfm$^6$) | 700 | | | | | | |
| MD (%) | 2.98 | | | | | | |
| $> 2M_\odot$ | no | yes | yes | yes | yes | yes | yes |
| J0740+6620 | $2\sigma$ | $1\sigma$ | $1\sigma$ | $1\sigma$ | $1\sigma$ | $1\sigma$ | $1\sigma$ |

TABLE XVII. Same as Table I, but for KIDS-D-Y4-LL4($\lambda_2$,800).

| | KIDS-D-Y4-LL4($\lambda_2$,800) | | | | | | |
|---|---|---|---|---|---|---|---|
| $\lambda_0$ (MeVfm$^3$) | −414.26 | | | | | | |
| $\lambda_1$ (MeVfm$^5$) | 432.20 | | | | | | |
| $\lambda_2$ (MeVfm$^5$) | 0 | 100 | 200 | 300 | 400 | 500 | 600 |
| $\lambda_3$ (MeVfm$^6$) | 800 | | | | | | |
| MD (%) | 3.10 | | | | | | |
| $> 2M_\odot$ | no | yes | yes | yes | yes | yes | yes |
| J0740+6620 | $2\sigma$ | $1\sigma$ | $1\sigma$ | $1\sigma$ | $1\sigma$ | $1\sigma$ | $1\sigma$ |

TABLE XVIII. Same as Table I, but for KIDS-D-Y4-LL4($\lambda_2$,900).

| | KIDS-D-Y4-LL4($\lambda_2$,900) | | | | | | |
|---|---|---|---|---|---|---|---|
| $\lambda_0$ (MeVfm$^3$) | $-435.03$ | | | | | | |
| $\lambda_1$ (MeVfm$^5$) | 448.71 | | | | | | |
| $\lambda_2$ (MeVfm$^5$) | 0 | 100 | 200 | 300 | 400 | 500 | 600 |
| $\lambda_3$ (MeVfm$^6$) | 900 | | | | | | |
| MD (%) | 3.22 | | | | | | |
| $> 2M_\odot$ | no | yes | yes | yes | yes | yes | yes |
| J0740+6620 | $2\sigma$ | $1\sigma$ | $1\sigma$ | $1\sigma$ | $1\sigma$ | $1\sigma$ | $1\sigma$ |

TABLE XIX. Same as Table I, but for KIDS-D-Y4-LL4($\lambda_2$,1000).

| | KIDS-D-Y4-LL4($\lambda_2$,1000) | | | | | | |
|---|---|---|---|---|---|---|---|
| $\lambda_0$ (MeVfm$^3$) | $-455.86$ | | | | | | |
| $\lambda_1$ (MeVfm$^5$) | 465.47 | | | | | | |
| $\lambda_2$ (MeVfm$^5$) | 0 | 100 | 200 | 300 | 400 | 500 | 600 |
| $\lambda_3$ (MeVfm$^6$) | 1000 | | | | | | |
| MD (%) | 3.33 | | | | | | |
| $> 2M_\odot$ | no | yes | yes | yes | yes | yes | yes |
| J0740+6620 | $2\sigma$ | $1\sigma$ | $1\sigma$ | $1\sigma$ | $1\sigma$ | $1\sigma$ | $1\sigma$ |

## II. NEUTRON-STAR PROPERTIES

Figs. 1–4 show (a) the mass–radius (M–R) relations, (b) the speed of sound as a function of the baryon density $\rho_B$, and (c) the $\Lambda$-hyperon fractions at the centers of neutron stars for the KIDS-A-Y4-LL4($\lambda_2, \lambda_3$) parameter sets.

Figs. 5-10 show the same plots as in Figs. 1-4, but for KIDS-D-Y4-LL4($\lambda_2, \lambda_3$) parameter sets.

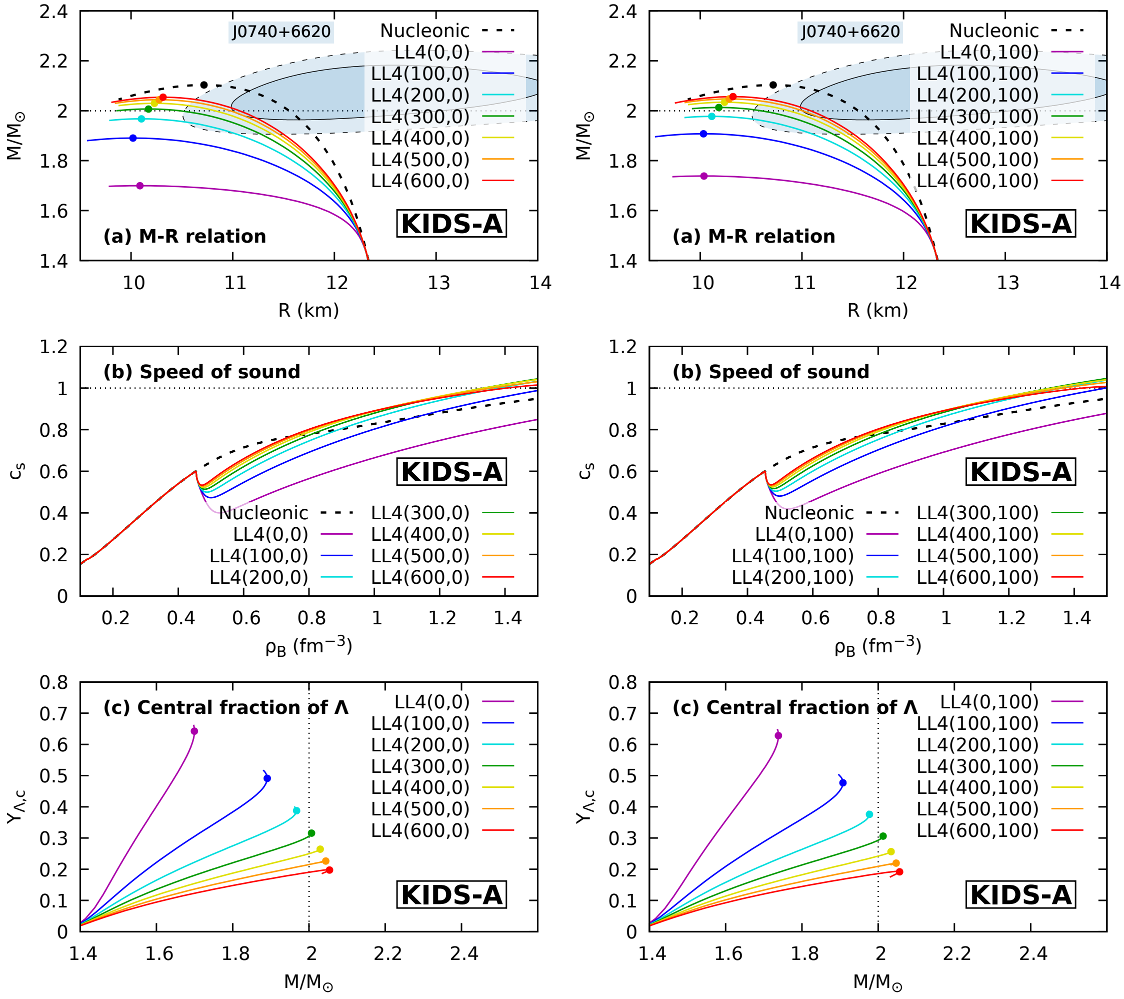


FIG. 1. Left: KIDS-A-Y4-LL4($\lambda_2$, 0) parameter sets. Right: KIDS-A-Y4-LL4($\lambda_2$, 100) parameter sets.

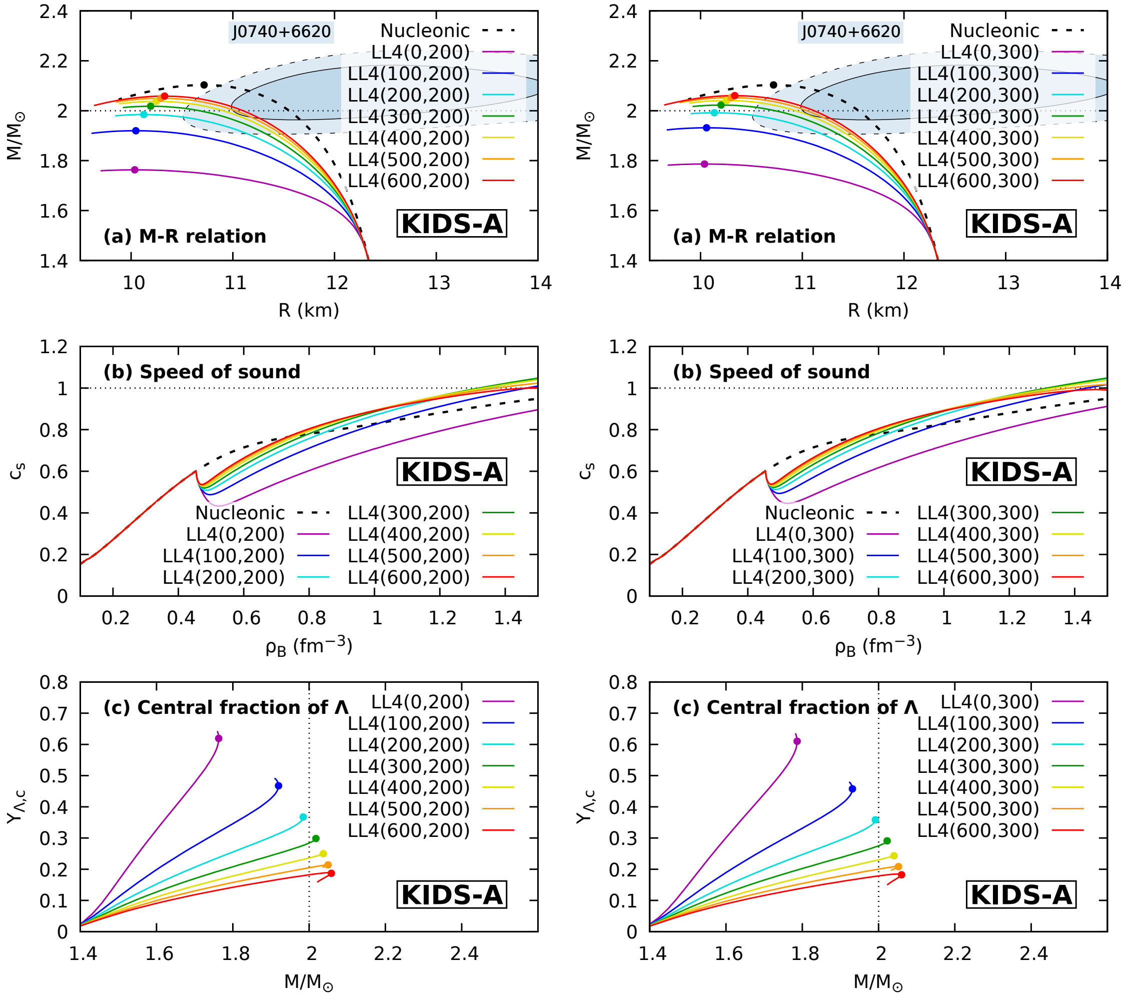


FIG. 2. Left: KIDS-A-Y4-LL4($\lambda_2, 200$) parameter sets. Right: KIDS-A-Y4-LL4($\lambda_2, 300$) parameter sets.

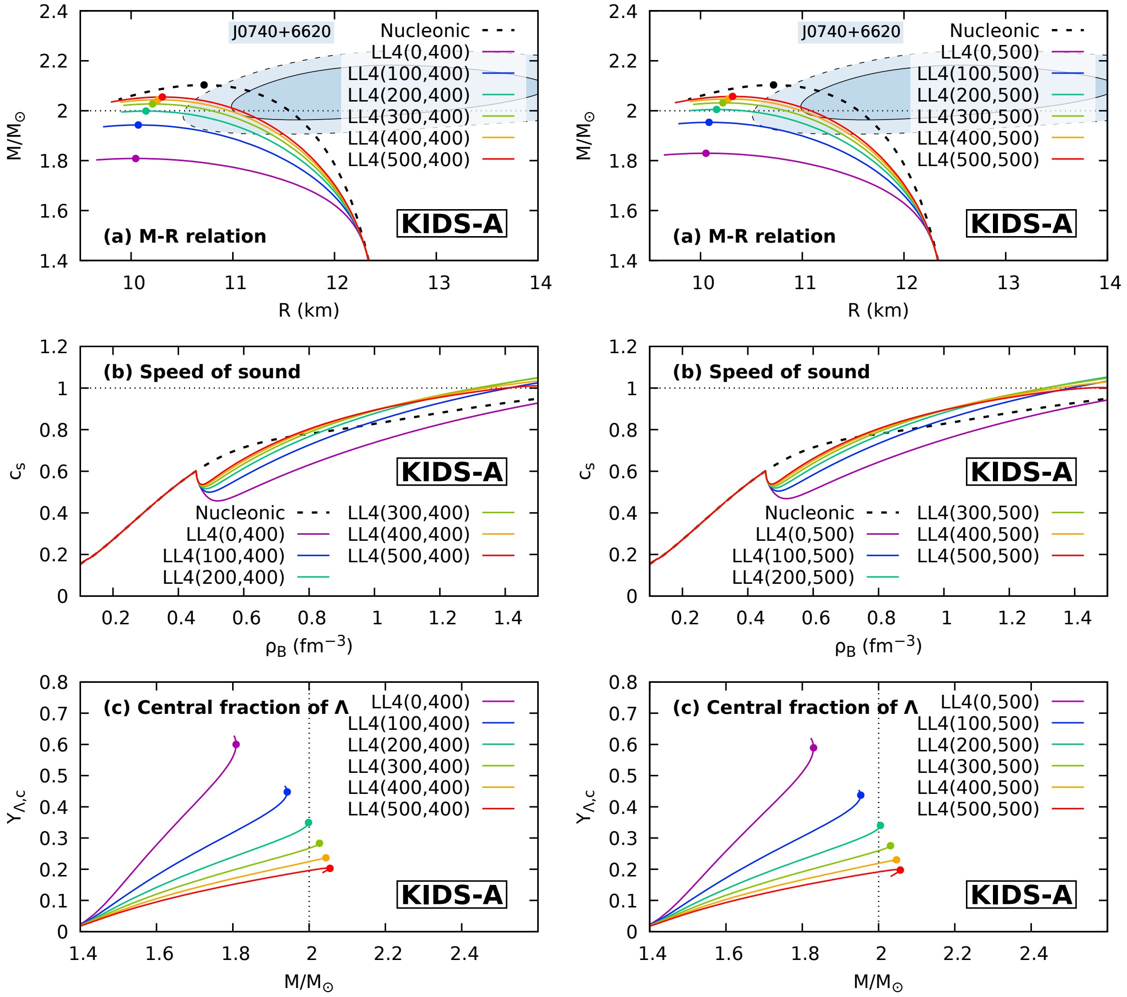


FIG. 3. Left: KIDS-A-Y4-LL4($\lambda_2$, 400) parameter sets. Right: KIDS-A-Y4-LL4($\lambda_2$, 500) parameter sets.

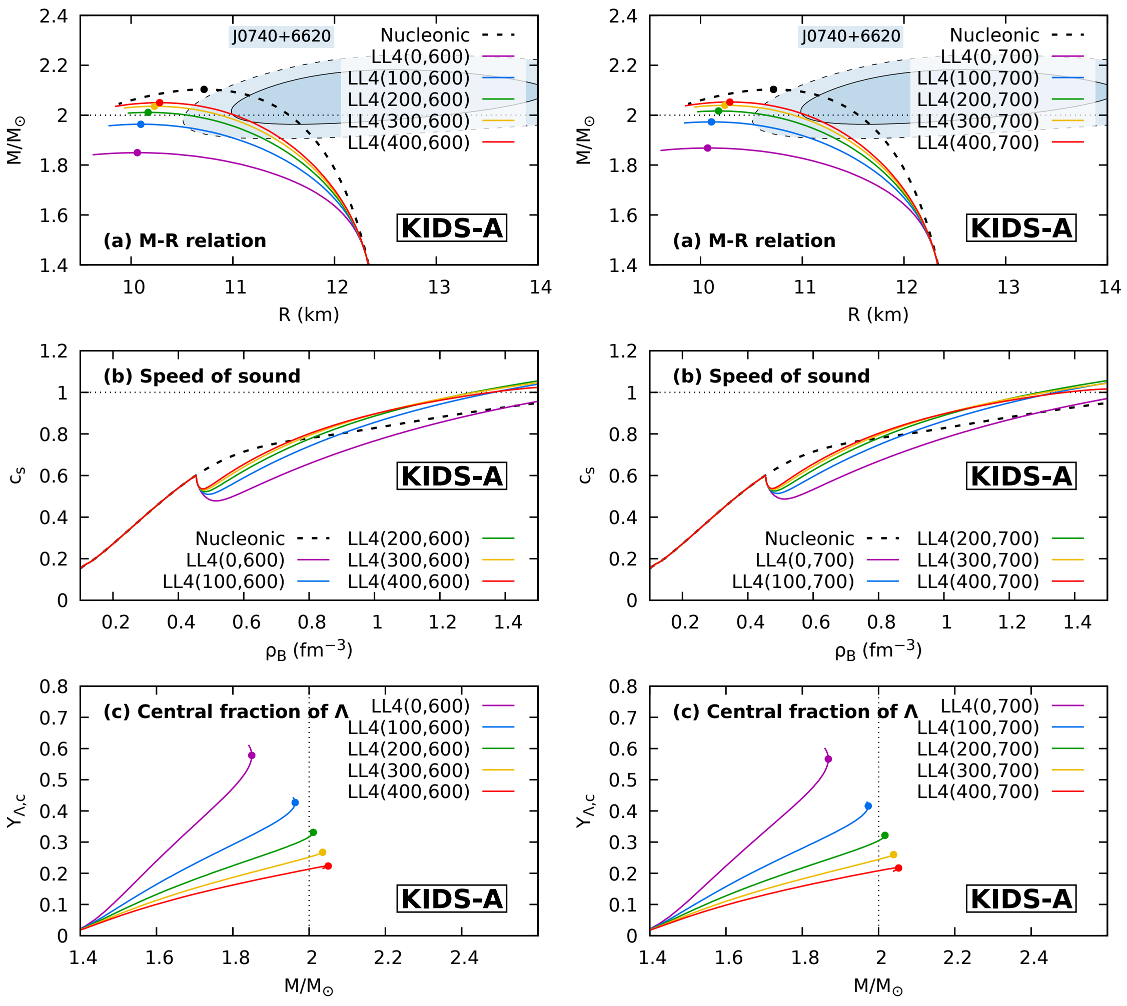


FIG. 4. Left: KIDS-A-Y4-LL4($\lambda_2, 600$) parameter sets. Right: KIDS-A-Y4-LL4($\lambda_2, 700$) parameter sets.

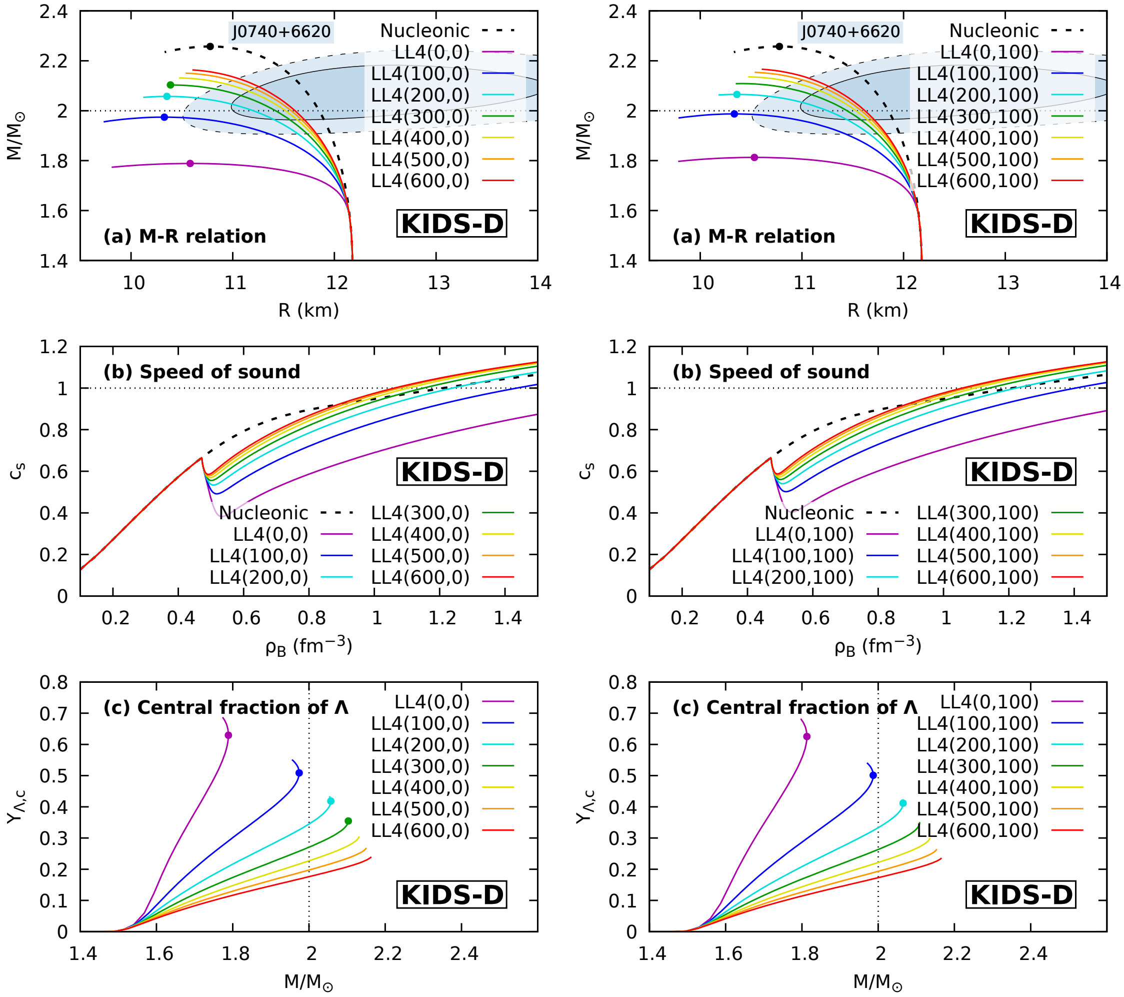


FIG. 5. Left: KIDS-D-Y4-LL4($\lambda_2, 0$) parameter sets. Right: KIDS-D-Y4-LL4($\lambda_2, 100$) parameter sets.

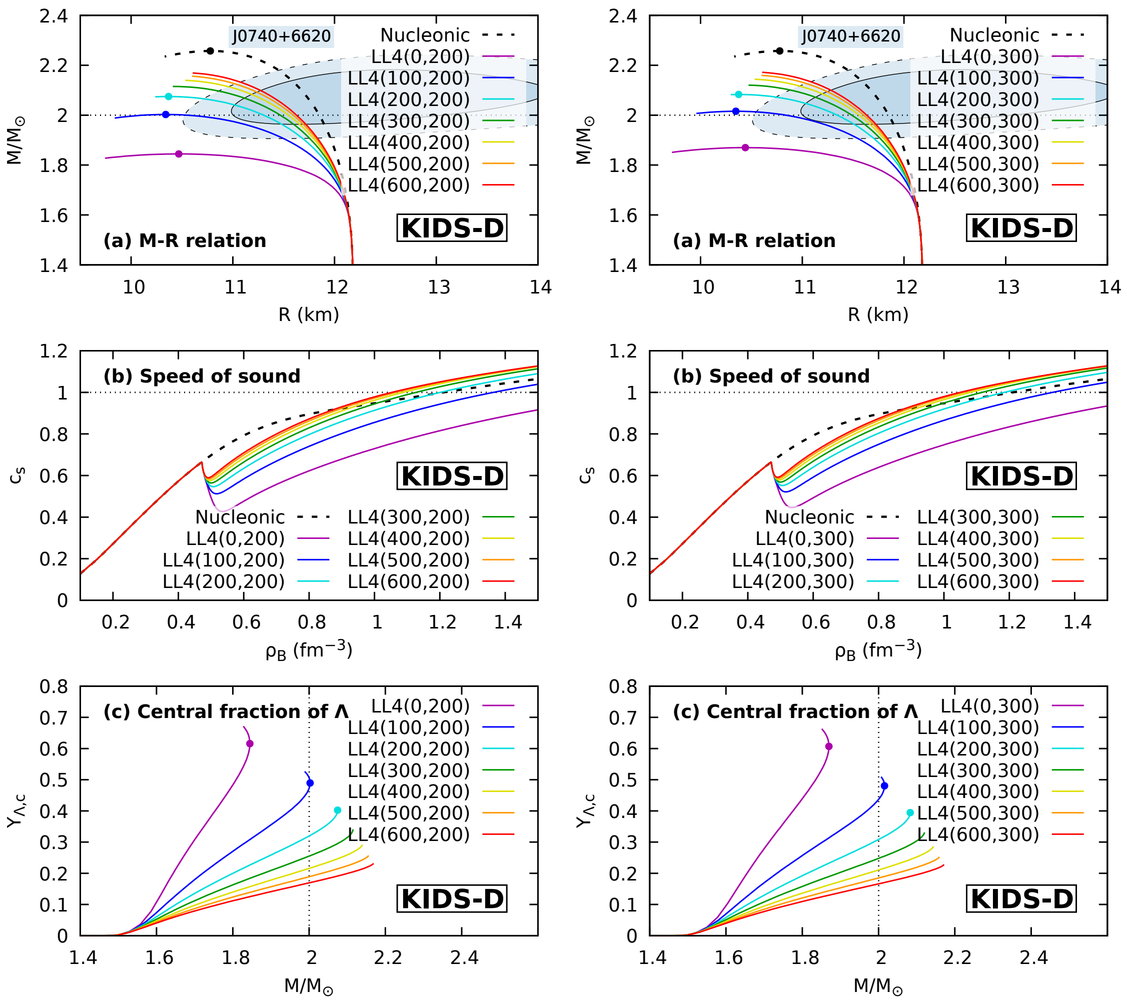


FIG. 6. Left: KIDS-D-Y4-LL4($\lambda_2, 200$) parameter sets. Right: KIDS-D-Y4-LL4($\lambda_2, 300$) parameter sets.

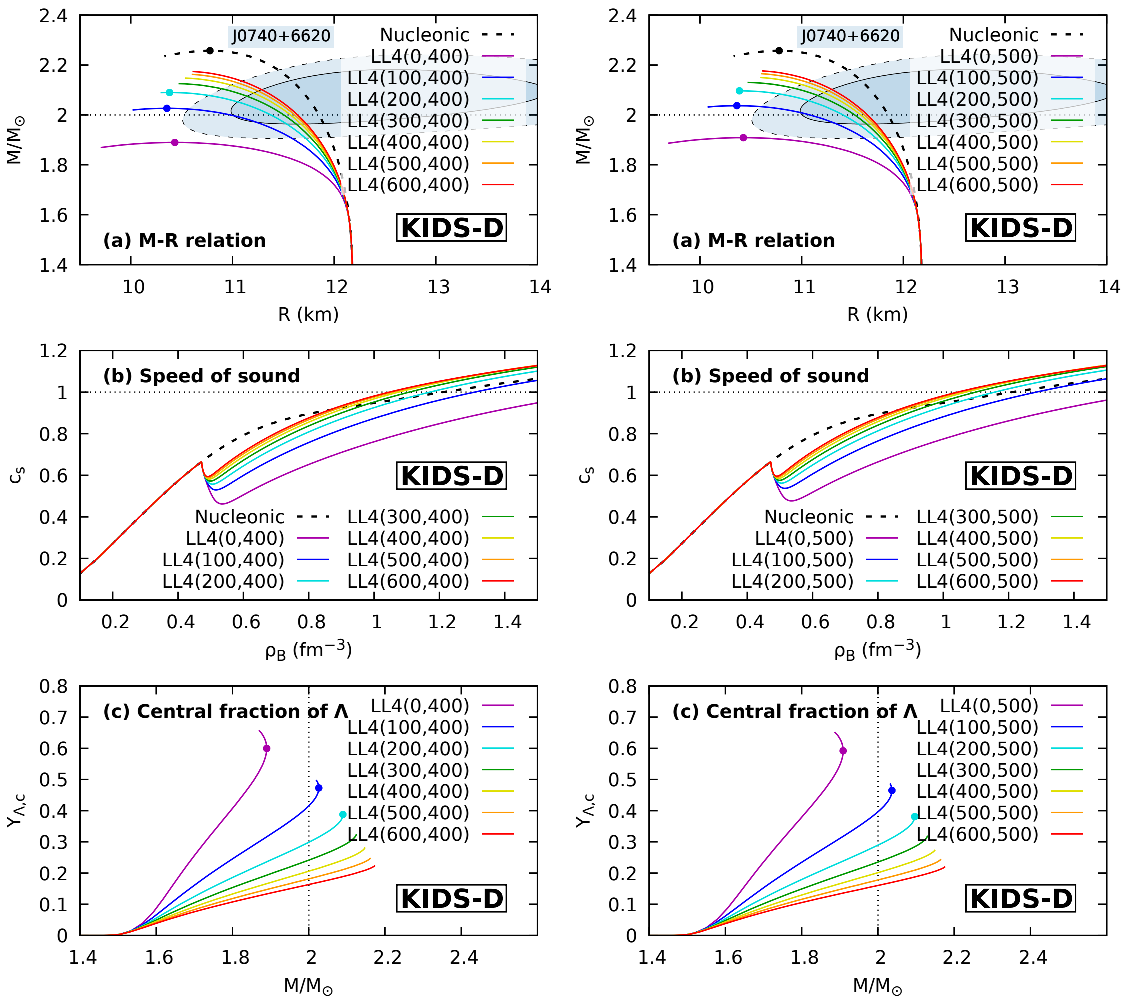


FIG. 7. Left: KIDS-D-Y4-LL4($\lambda_2, 400$) parameter sets. Right: KIDS-D-Y4-LL4($\lambda_2, 500$) parameter sets.

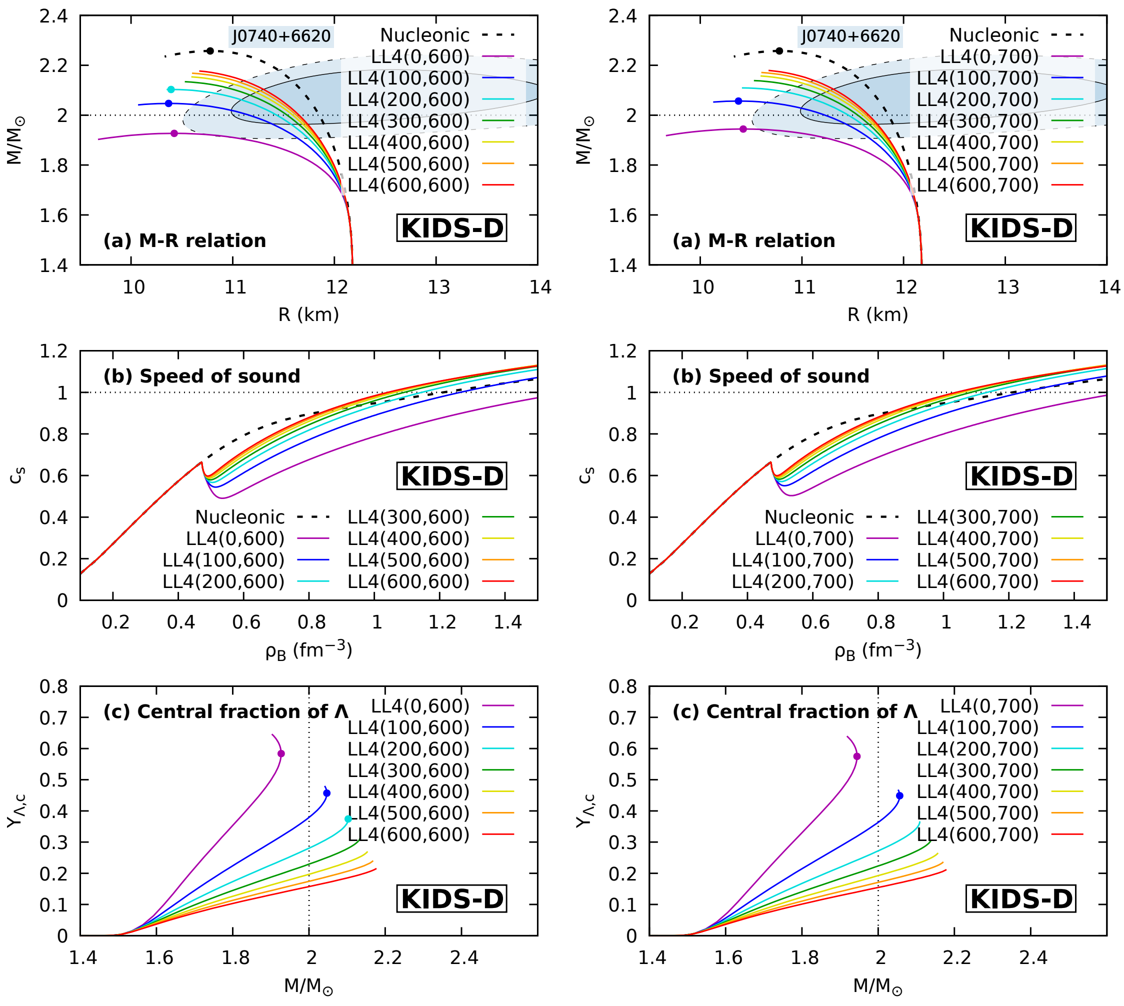


FIG. 8. Left: KIDS-D-Y4-LL4($\lambda_2, 600$) parameter sets. Right: KIDS-D-Y4-LL4($\lambda_2, 700$) parameter sets.

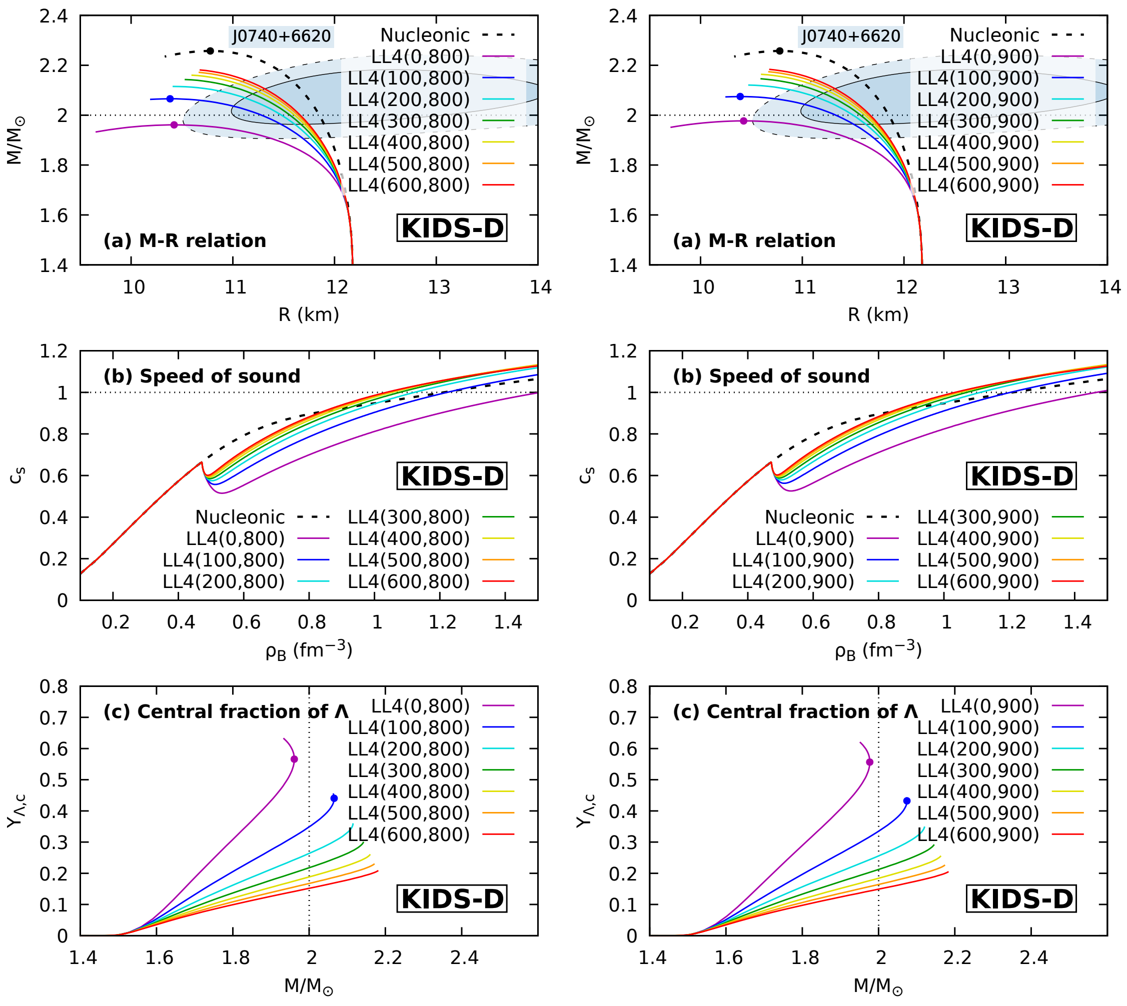


FIG. 9. Left: KIDS-D-Y4-LL4($\lambda_2, 800$) parameter sets. Right: KIDS-D-Y4-LL4($\lambda_2, 900$) parameter sets.

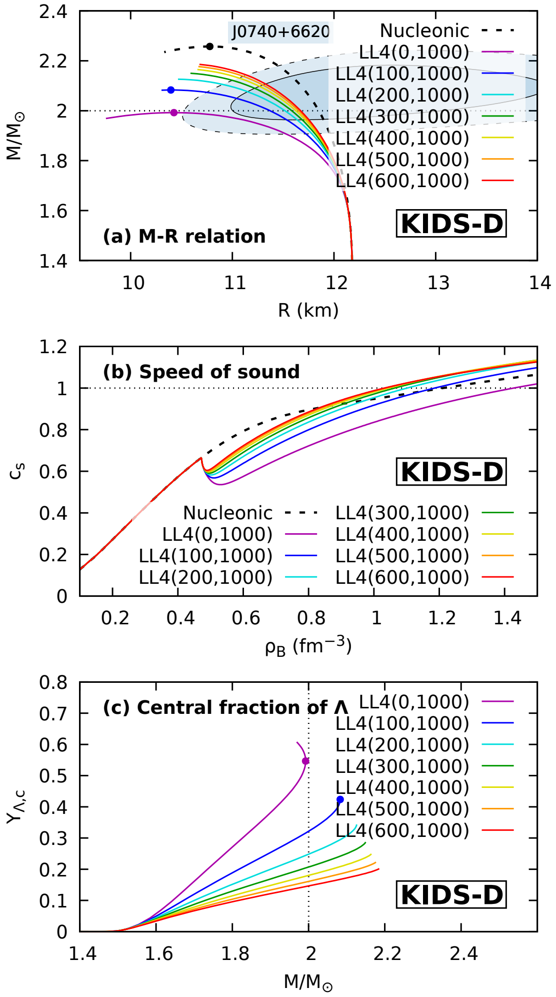


FIG. 10. KIDS-D-Y4-LL4($\lambda_2, 1000$) parameter sets.

[1] Tuomo Salmi *et al.*, The Radius of the High-mass Pulsar PSR J0740+6620 with 3.6 yr of NICER Data, Astrophysical Journal **974**, 294 (2024).

[2] Tuomo Salmi *et al.*, Data and Software for: 'The Radius of the High-mass Pulsar PSR J0740+6620 with 3.6 yr of NICER Data', Version 1.0.0, Zenodo (2024).
